# Supplementary material for: New routes for PN destruction and formation in the ISM via neutral-neutral gas-phase reactions and an extended database for reactions involving phosphorus
Source: arXiv:2503.03635 source file (2025-03-05)
Supplement: Supplementary file 1 [file Supp_Info.pdf]

# New routes for PN destruction and formation in the ISM via neutral-neutral gas-phase reactions and an extended database for reactions involving phosphorus

Mateus X. Silva[1], Edgar Mendoza[2], Fábio S. L. Ferreira[3], Alexandre C. R. Gomes[3,5], Miguel Carvajal[2,4], Jing Li[5], António J. C. Varandas[1,5,6] and Breno R. L. Galvão[3]

[1] Departamento de Física, Universidade Federal do Espírito Santo, Av. Fernando Ferrari 514, Vitória, ES, 29075-910, Brazil.

[2] Dept. Ciencias Integradas, Facultad de Ciencias Experimentales, Centro de Estudios Avanzados en Física, Matemática y Computación, Unidad Asociada GIFMAN, CSIC-UHU, Universidad de Huelva, Spain. e-mail: edgar.mendoza@dci.uhu.es

[3] Departamento de Química, Centro Federal de Educação Tecnológica de Minas Gerais, Av. Amazonas 5253, Belo Horizonte, MG, 30421-169, Brazil. e-mail: brenogalvao@gmail.com

[4] Instituto Universitario "Carlos I" de Física Teórica y Computacional, Universidad de Granada, Spain.

[5] School of Physics and Physical Engineering Qufu Normal University, Qufu, Shandong 273165, China.

[6] Coimbra Chemistry Centre and Chemistry Department, University of Coimbra, 3004-535 Coimbra, Portugal.

## Supplementary Information

***Part I,*** *Rate coefficients of the PO + N → PN + O and PO + N → NO + P reactions.*

***Part II,*** *CASSCF/aug-cc-pV(T+d)Z geometries and frequencies.*

***Part III,*** *M06-2X/aug-cc-pV(T+d)Z geometries and frequencies.*

# Part I

## Rate coefficients of the PO + N $\rightarrow$ PN + O and PO + N $\rightarrow$ NO + P reactions

We have calculated the rate coefficient of an important reaction of the PNO triatomic system using the MESS software package and employing the same methodology described in section 2.2 of the main document of the present work. The studied reaction was the following:

$$PO + N \rightarrow PN + O \qquad (S1)$$

Its rate coefficient as a function of temperature was obtained in the present work based on accurate computations at the MRCI(Q)/AV(5+d)Z//CAS/AV(5+d)Z + ZPE(CAS/AV(5+d)Z) level carried out in our previous work on the PNO system (Souza et al. 2021). The reader is referred to the potential energy profile shown in Figure 2 of the cited reference, which shows a barrierless path in the entrance channel of the PO + N reaction. The calculated rate coefficients for several different temperatures were then fitted to the modified Arrhenius equation.

The $^3A'$ and $^3A''$ electronic states were taken into consideration separately and their individual contributions were then added to provide the total value of the rate coefficient.

The electronic degeneracy of the oxygen atom in the $^3P$ state was taken into consideration according to the splitting of the ground energy level due to spin-orbit coupling as available in NIST Atomic Spectra Database (Kramida et al. 2024). This interaction gives rise to three finely separated energy levels with total angular momentum quantum number $J$ = 2, 1 and 0 and electronic degeneracy number $g$ = 5, 3 and 1, respectively. The ground state corresponds to $J$ = 2, while the states with $J$ = 1 and 0 lie 158.3 and 227.0 $cm^{-1}$ above it, respectively. For the PO ($^2\Pi$) molecule, the electronic ground state splits into two doubly degenerate levels with energy separation of 223.8 $cm^{-1}$, according to Herzberg, G. (1950).

As for the PO + N → P + NO reaction, despite also showing a barrierless path in the entrance channel, a crossing between the ground $^3A'$ state and the excited one of the same symmetry occurs on the pathway that leads to P + NO formation. Thus, we did not calculate the rate coefficient for this reaction. However, due to the occurrence of this conical intersection on the potential energy surface outlined in Figure 2 of our previous work (Souza et al. 2021), it is plausible to estimate its rate coefficient to be about one order of magnitude lower than that of reaction S1. Therefore, the estimate available in KIDA and UMIST should be reasonable and was kept in table 3 of the main document of the present work. We did not employ the rate coefficient provided in the work of Douglas et al. 2022 for this reaction, since it does not consider the barrierless isomerization pathway involving the conical intersection. Rather, it only considers the PO + N → PON → P + NO abstraction mechanism which, according to our calculations, presents both high entrance and exit barriers. All the other chemical reactions within the PNO system present either an entrance or an exit energy barrier.

## References


Douglas, K. M., Gobrecht, D., & Plane, J. M. C. 2022, MNRAS, 515, 99.

Herzberg, G. Molecular Spectra and Molecular Structure. I. Spectra of Diatomic Molecules, Van Nostrand, Princeton, 2nd Ed, 1950.

Kramida, A., Ralchenko, Yu., Reader, J., & NIST ASD Team (2024). NIST Atomic Spectra Database (ver. 5.12), [Online]. Available: https://physics.nist.gov/asd [2025, February 9]. National Institute of Standards and Technology, Gaithersburg, MD.

Souza, A. C., Silva, M. X., & Galvão, B. R. L. 2021, MNRAS, 507, 1899.

# Part II

Structures and frequencies obtained at the CASSCF/aug-cc-pV(T+d)Z level

(Coordinates in Ångstrom and frequencies in $cm^{-1}$)

Optimized Cartesian coordinates (Å) and vibrational frequencies ($cm^{-1}$) for all structures obtained in this work at the CASSCF/AV(T+d)Z level.

2

PN $^1\Sigma^+$

| | | | |
|---|---|---|---|
| P | -0.7198241757 | 0.0326972275 | 0.0000000000 |
| N | 0.7842283657 | 0.1101571925 | 0.0000000000 |

1314.90

---

2

CP $^2\Sigma^+$

| | | | |
|---|---|---|---|
| C | 0.4973370561 | -0.1808135097 | 0.0000000000 |
| P | -1.0789015561 | -0.1057545203 | 0.0000000000 |

1216.62

---

2

CN $^2\Sigma^+$

| | | | |
|---|---|---|---|
| C | 0.0086836316 | -0.1364679972 | 0.0000000000 |
| N | -1.1718125816 | -0.1753854528 | 0.0000000000 |

2038.16

---

2

CN $^2\Pi$

| | | | |
|---|---|---|---|
| C | 0.0406807748 | -0.1354131464 | 0.0000000000 |
| N | -1.2038097248 | -0.1764403036 | 0.0000000000 |

1778.23

---

3

CNP $^3A'$

| | | | |
|---|---|---|---|
| C | 0.0000000000 | 0.3415403130 | -1.6739208417 |

| | | | |
|---|---|---|---|
| N | 0.0000000000 | -0.5130004533 | -0.5670918067 |
| P | 0.0000000000 | 0.0995424110 | 0.9055583836 |

330.22
650.35
993.72

---

3

CPN $^3A''$

| | | | |
|---|---|---|---|
| C | 0.0000000000 | 0.1688729223 | -1.7495699179 |
| P | 0.0000000000 | -0.1413111290 | -0.0026254425 |
| N | 0.0000000000 | 0.1676772062 | 1.5060938059 |

96.11
622.28
1084.33

---

3

CNP $^3A''$

| | | | |
|---|---|---|---|
| C | 0.0000000000 | 0.0000013245 | -1.8651740304 |
| N | 0.0000000000 | -0.0000019317 | -0.6732497498 |
| P | 0.0000000000 | 0.0000003599 | 1.0277283917 |

245.00
245.00
657.45
2005.17

---

3

NCP $^3A''$

| | | | |
|---|---|---|---|
| N | 0.0000000000 | -0.0000005286 | -1.8489392588 |
| C | 0.0000000000 | 0.0000010278 | -0.6701776878 |
| P | 0.0000000000 | -0.0000001595 | 1.0959935676 |

316.91
316.92
609.36
2051.32

---

3

$TS_{C+PN \rightarrow CNP}$ $^3A'$

| | | | |
|---|---|---|---|
| C | 0.0000000000 | 0.3331502359 | -2.0904373755 |
| N | 0.0000000000 | -0.6791198163 | -0.3246874962 |
| P | 0.0000000000 | 0.1779170513 | 0.9574570110 |

828.50 i
249.00
1104.11

---

3

$TS_{CNP \rightarrow NCP}$ $^3A''$

| | | | |
|---|---|---|---|
| N | 0.0000000000 | 0.5465001745 | -1.0650462265 |
| C | 0.0000000000 | -0.6593275257 | -1.0004255517 |
| P | 0.0000000000 | 0.0085400970 | 0.8695713495 |

305.41 i
465.85
1883.87

---

3

$TS_{CPN \rightarrow CNP}$ $^3A''$

| | | | |
|---|---|---|---|
| C | 0.0000000000 | 0.5626660902 | -1.4398051484 |
| P | 0.0000000000 | -0.4575986550 | -0.0188087820 |
| N | 0.0000000000 | 0.5294158159 | 1.2762519607 |

684.76 i
630.04
847.09

---

3

$TS_{CPN \rightarrow N+CP}$ $^3A''$

| | | | |
|---|---|---|---|
| N | 0.0000000000 | 0.0000000000 | -2.2247436878 |
| P | 0.0000000000 | 0.0000000000 | 0.2797950222 |
| C | 0.0000000000 | 0.0000000000 | 1.8728676667 |

378.93 i
80.52
81.16
1094.93

---

# Part III

## Structures and frequencies obtained at the M06-2X/aug-cc-pV(T+d)Z level

(Coordinates in Ångstrom and frequencies in $cm^{-1}$)

Optimized Cartesian coordinates (Å) and vibrational frequencies ($cm^{-1}$) for all structures obtained in this work at the M06-2X/AV(T+d)Z level.

2

PN $^1\Sigma^+$

| | | | |
|---|---|---|---|
| P | -0.7027817379 | 0.0335749273 | 0.0000000000 |
| N | 0.7671859279 | 0.1092794927 | 0.0000000000 |

1468.97

---

2

CP $^2\Sigma^+$

| | | | |
|---|---|---|---|
| C | 0.4792358116 | -0.1799515455 | 0.0000000000 |
| P | -1.0608003116 | -0.1066164845 | 0.0000000000 |

1330.59

---

2

CN $^2\Sigma^+$

| | | | |
|---|---|---|---|
| C | -0.0056477488 | -0.1369404603 | 0.0000000000 |
| N | -1.1574812012 | -0.1749129897 | 0.0000000000 |

2238.78

---

3

CNP $^3A'$

| | | | |
|---|---|---|---|
| C | 0.0000000000 | 0.3334664637 | -1.6410466703 |
| N | 0.0000000000 | -0.4978154447 | -0.5633917553 |
| P | 0.0000000000 | 0.0958064469 | 0.8911372354 |

368.77
1016.75
1256.88

---

3

CPN $^3A''$

| | | | |
|---|---|---|---|
| C | 0.0000000000 | 0.0000000000 | -1.7407828963 |
| P | 0.0000000000 | 0.0000000000 | -0.0040572057 |
| N | 0.0000000000 | 0.0000000000 | 1.5017249090 |

216.14
244.35
637.05
1213.09

---

3

CNP $^3A''$

| | | | |
|---|---|---|---|
| C | 0.0000000000 | 0.0000000000 | -1.8352087525 |
| N | 0.0000000000 | 0.0000000000 | -0.6546891977 |
| P | 0.0000000000 | 0.0000000000 | 1.0077151599 |

269.83
269.83
709.29
2050.28

---

3

NCP $^3A''$

| | | | |
|---|---|---|---|
| N | 0.0000000000 | 0.0000000000 | -1.8165025765 |
| C | 0.0000000000 | 0.0000000000 | -0.6561109847 |
| P | 0.0000000000 | 0.0000000000 | 1.0758705329 |

333.56
333.56
653.19
2152.24

---

3

$TS_{C+PN \rightarrow CNP}$ $^3A'$

| | | | |
|---|---|---|---|
| C | 0.0000000000 | 0.3096086696 | -2.1809481591 |
| N | 0.0000000000 | -0.6916751577 | -0.2471720184 |
| P | 0.0000000000 | 0.1927236700 | 0.9575018548 |

511.37 i
208.63
1294.57

---

3

$TS_{CNP \rightarrow NCP}$ $^{3}A''$

| | | | |
|---|---|---|---|
| C | 0.0000000000 | 0.6504790461 | -0.8372707599 |
| N | 0.0000000000 | -0.4477354925 | -1.2632239980 |
| P | 0.0000000000 | -0.0497914329 | 0.8958176772 |

349.77 i
628.22
2047.68

---

3

$TS_{CPN \rightarrow CNP}$ $^{3}A''$

| | | | |
|---|---|---|---|
| C | 0.0000000000 | 0.5670315343 | -1.3710900863 |
| P | 0.0000000000 | -0.4370407760 | -0.0503247503 |
| N | 0.0000000000 | 0.4802116379 | 1.2870204805 |

384.91 i
746.22
984.29

---

3

$TS_{CPN \rightarrow N+CP}$ $^{3}A''$

| | | | |
|---|---|---|---|
| C | 0.0000000000 | -0.2988163611 | -1.6591762833 |
| P | 0.0000000000 | 0.5132045346 | -0.3268999750 |
| N | 0.0000000000 | -0.2166851184 | 2.0047927810 |

276.12 i
76.20
1174.43

---
